# Supplementary material for: Rethinking Stateful Tool Use in Multi-Turn Dialogues: Benchmarks and Challenges
Source: arXiv:2505.13328 source file (2025-05-19)
Supplement: Supplementary file 1 [file checklist.tex]

\newcommand{\answerYes}[1]{\textbf{\textcolor{blue}{#1}}}
\newcommand{\answerNo}[1]{\textbf{\textcolor{teal}{#1}}}
\newcommand{\answerNA}[1]{\textbf{\textcolor{gray}{#1}}}


\paragraph{This paper:}
\begin{itemize}
    \item Includes a conceptual outline and/or pseudocode description of AI methods introduced \answerYes{Yes} % (yes/partial/no/NA)
    \item Clearly delineates statements that are opinions, hypothesis, and speculation from objective facts and results \answerYes{Yes} %(yes/no)
    \item Provides well marked pedagogical references for less-familiare readers to gain background necessary to replicate the paper \answerYes{Yes} %(yes/no)
\end{itemize}


\paragraph{Does this paper make theoretical contributions? \answerNo{No}} %(yes/no)
% \emph{If yes, please complete the list below.}
% \begin{itemize}
%     \item All assumptions and restrictions are stated clearly and formally. (yes/partial/no)
%     \item All novel claims are stated formally (e.g., in theorem statements). (yes/partial/no)
%     \item Proofs of all novel claims are included. (yes/partial/no)
%     \item Proof sketches or intuitions are given for complex and/or novel results. (yes/partial/no)
%     \item Appropriate citations to theoretical tools used are given. (yes/partial/no)
%     \item All theoretical claims are demonstrated empirically to hold. (yes/partial/no/NA)
%     \item All experimental code used to eliminate or disprove claims is included. (yes/no/NA)
% \end{itemize}

\paragraph{Does this paper rely on one or more datasets? \answerYes{Yes}} %(yes/no)
% If yes, please complete the list below.
\begin{itemize}
    \item A motivation is given for why the experiments are conducted on the selected datasets \answerYes{Yes} %(yes/partial/no/NA)
    \item All novel datasets introduced in this paper are included in a data appendix. \answerNo{No} %(yes/partial/no/NA)
    \item All novel datasets introduced in this paper will be made publicly available upon publication of the paper with a license that allows free usage for research purposes. \answerYes{Yes} %(yes/partial/no/NA)
    \item All datasets drawn from the existing literature (potentially including authors’ own previously published work) are accompanied by appropriate citations. \answerYes{Yes} % (yes/no/NA)
    \item All datasets drawn from the existing literature (potentially including authors’ own previously published work) are publicly available. \answerYes{Yes} % (yes/partial/no/NA)
    \item All datasets that are not publicly available are described in detail, with explanation why publicly available alternatives are not scientifically satisficing. \answerNA{NA, we do not use datasets that are not publicly available.} %(yes/partial/no/NA)
\end{itemize}

\paragraph{Does this paper include computational experiments? \answerYes{Yes}} %(yes/no)
% If yes, please complete the list below.
\begin{itemize}
    \item Any code required for pre-processing data is included in the appendix. \answerYes{Partial}.
    \item All source code required for conducting and analyzing the experiments is included in a code appendix. \answerNo{No}
    \item All source code required for conducting and analyzing the experiments will be made publicly available upon publication of the paper with a license that allows free usage for research purposes. \answerYes{Yes} %(yes/partial/no)
    \item All source code implementing new methods have comments detailing the implementation, with references to the paper where each step comes from \answerYes{Yes} %(yes/partial/no)
    \item If an algorithm depends on randomness, then the method used for setting seeds is described in a way sufficient to allow replication of results. \answerYes{Yes} %(yes/partial/no/NA)
    \item This paper specifies the computing infrastructure used for running experiments (hardware and software), including GPU/CPU models; amount of memory; operating system; names and versions of relevant software libraries and frameworks. \answerYes{Yes} %(yes/partial/no)
    \item This paper formally describes evaluation metrics used and explains the motivation for choosing these metrics. \answerYes{Yes} %(yes/partial/no)
    \item This paper states the number of algorithm runs used to compute each reported result. \answerYes{Yes} %(yes/no)
    \item Analysis of experiments goes beyond single-dimensional summaries of performance (e.g., average; median) to include measures of variation, confidence, or other distributional information. \answerNo{No} %(yes/no)
    \item The significance of any improvement or decrease in performance is judged using appropriate statistical tests (e.g., Wilcoxon signed-rank). \answerNo{No} %(yes/partial/no)
    \item This paper lists all final (hyper-)parameters used for each model/algorithm in the paper’s experiments. \answerYes{Yes} %(yes/partial/no/NA)
    \item This paper states the number and range of values tried per (hyper-) parameter during development of the paper, along with the criterion used for selecting the final parameter setting. \answerNA{NA, we basically using greedy decoding to evaluate the performance.} %(yes/partial/no/NA)
\end{itemize}
